# Supplementary material for: In Defense of Lazy Visual Grounding for Open-Vocabulary Semantic Segmentation
Source: arXiv:2408.04961 source file (2024-08-09)
Supplement: Supplementary file 1 [file 32masks.tex]

\begin{table*}[t!]
    \centering
    \caption{Ablation study of LaVG on the object mask discovery models}
    \label{table:32masks}
    \tabcolsep=0.04cm
    \scalebox{0.92}{
    \begin{tabular}{lcccccc}
    \toprule
    % & \multicolumn{3}{c}{\it With a background category} & \multicolumn{3}{c}{\it Without background category} \\\cmidrule(lr){2-4}\cmidrule(lr){5-7}
    & VOC21 & Context60 & COCO-Obj. & VOC20 & Context59  & COCO-Stf. \\\midrule
    Normalized cut~\cite{normalizedcut} & 47.6 & 26.3 & 28.2 & 78.1 & 29.3 & 20.0 \\ 
    CutLER-CascadedRCNN~\cite{cutler} & 57.3 & 29.3 & 33.2 & 79.6 & 32.2 & 22.3 \\ 
    Panoptic cut (4 iterations) & 61.1 & 30.3 & 33.7 & 81.3 & 33.4 & 22.6 \\
        \rowcolor{gray!10}
    Panoptic cut (16 iterations) & \bf 61.7 & 31.6 & \bf 34.2 & 82.5 & \bf 34.8 & 23.2 \\ 
    Panoptic cut (32 iterations) & 61.4 & \bf 31.7 & \bf 34.2 & \bf 82.6 & \bf 34.8 & \bf 23.3 \\ 
    \gray{Ground-truth object masks} & \gray{68.3} & \gray{37.1} & \gray{44.1} & \gray{87.7} & \gray{40.2} & \gray{27.6} \\ \bottomrule
    \end{tabular}
    }
\end{table*}
