# Supplementary material for: In Defense of Lazy Visual Grounding for Open-Vocabulary Semantic Segmentation
Source: arXiv:2408.04961 source file (2024-08-09)
Supplement: Supplementary file 2 [file groundingbackbone.tex]

\begin{table*}[t!]
    \centering
    \caption{Results of our model with different backbones used for visual grounding}
    \label{table:groundingbackbone}
    \tabcolsep=0.04cm
    \scalebox{0.9}{
    \begin{tabular}{lccccccc}
    \toprule
    & VOC21 & Context60 & COCO-Obj. & VOC20 & Context59  & ADE & COCO-Stf. \\\midrule
    CLIP-L/14 & \gray{51.4} & \gray{24.5} & \gray{28.3} & \gray{78.5} & \gray{27.9} & \gray{12.1}  & \gray{18.7} \\ 
    % CLIP-L/14-336px & \gray{xx.x} & \gray{xx.x} & \gray{xx.x} & \gray{xx.x} & \gray{xx.x} & \gray{xx.x}  & \gray{xx.x} \\ 
    \rowcolor{gray!10}
    CLIP-B/16 & \bf 62.1 & \bf 31.6 & \bf 34.2 & \bf 82.5 & \bf 34.7 & 15.8 & \bf 23.2  \\ 
    \bottomrule
    \end{tabular}
    }
\end{table*}
